# Supplementary material for: Controllable Gradient Item Retrieval
Source: arXiv:2106.00062 source file (2021-05-31)
Supplement: Supplementary file 1 [file appendix.tex]

\section{appendix}

\subsection{Decomposition of KL-divergence}
